# Supplementary material for: Direct laser writing of high aspect ratio nanochannels for nanofluidics
Source: arXiv:2602.06316 ancillary file (2026-02-06)

Reflected light microscopy images of a nanochannel in the water- and air-filled states at each of the 100 fill and drain cycles. Each pair of images represents a cycle, and the channel appears most dark when it is filled with water (left). The channel is approximately 200  $\mu\text{m}$  long.

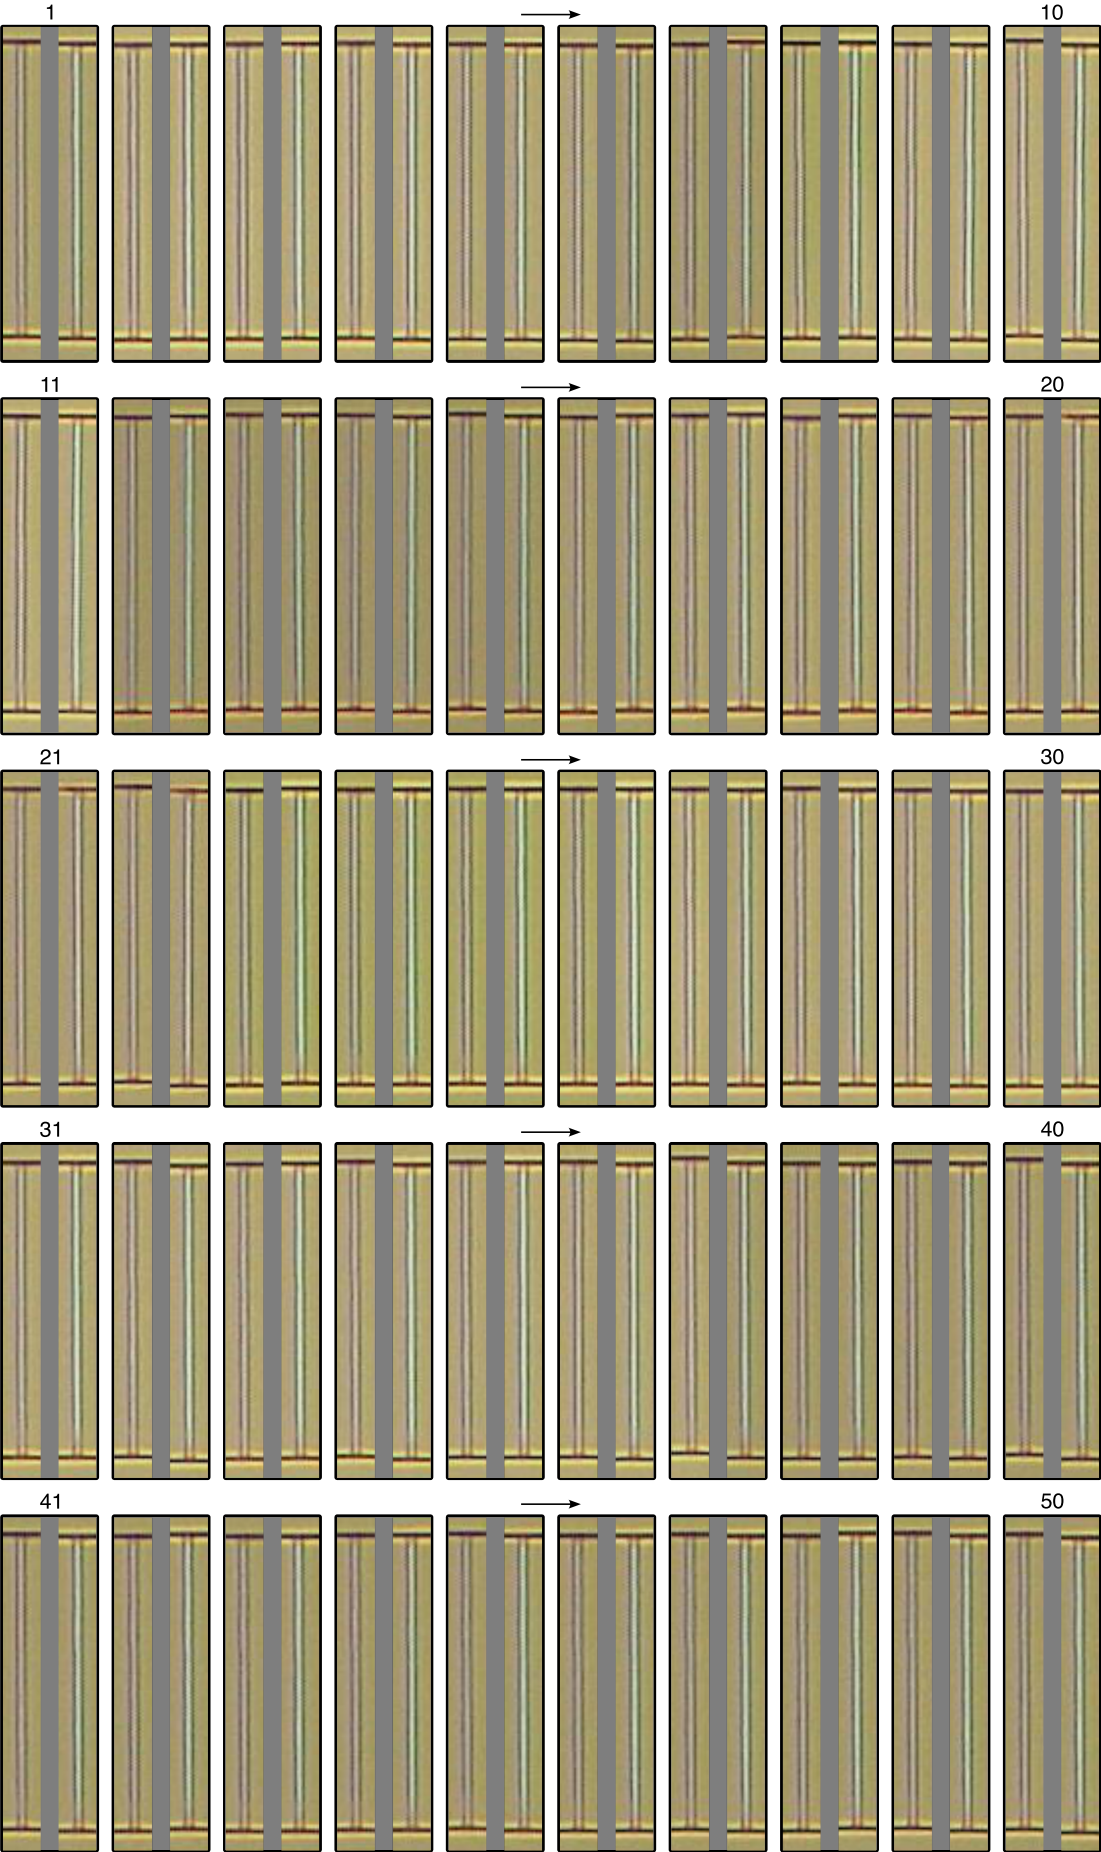

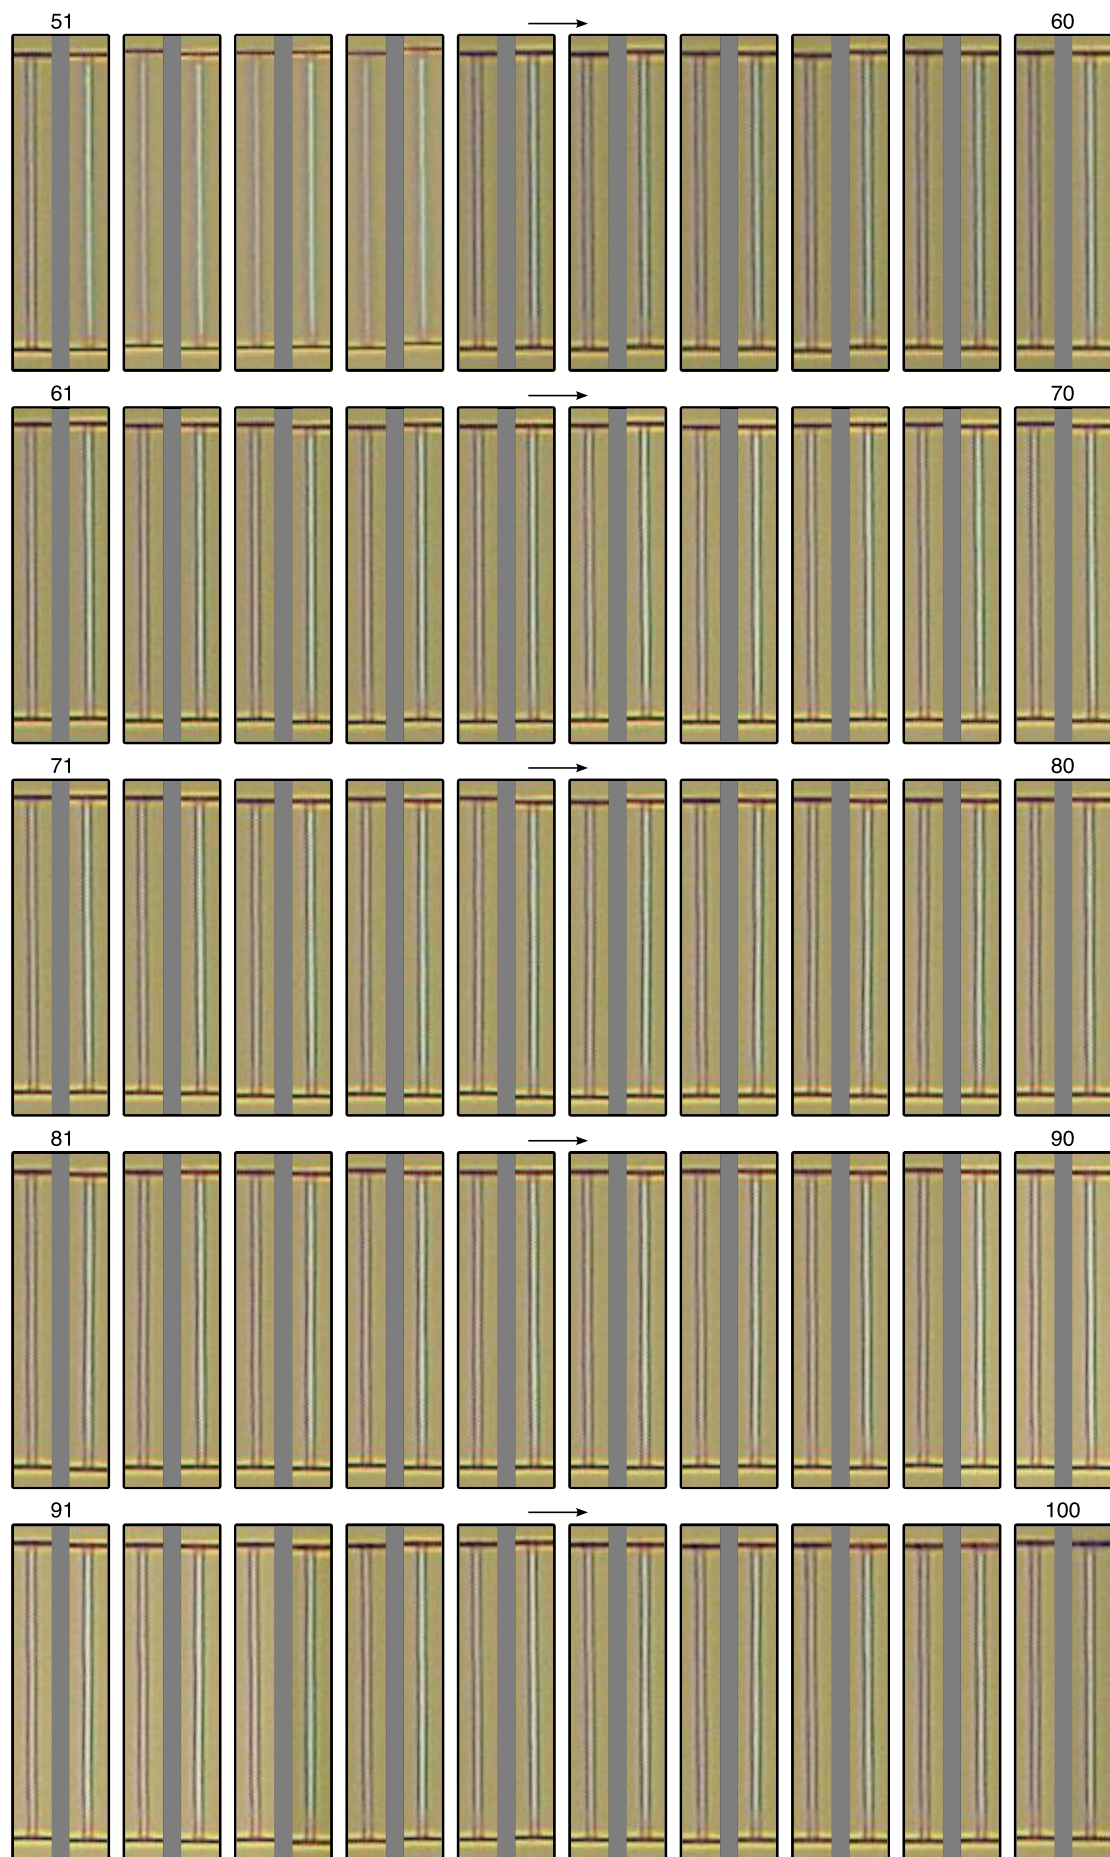

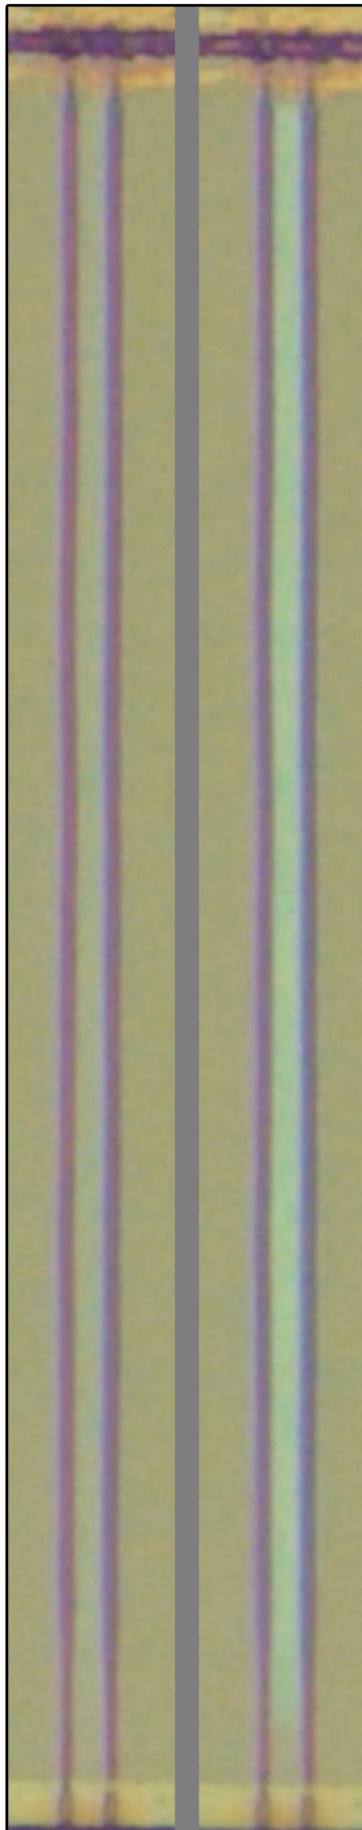

Supplement: Supplementary file 1 [file Supplementary_information.pdf]
